# Supplementary material for: Neural Approximation of an Auto-Regressive Process through Confidence Guided Sampling
Source: arXiv:1910.06705 source file (2019-10-15)
Supplement: Supplementary file 1 [file 9_Experiment_supp.tex]

\section{Supplementary Results}

\subsection{Parallel Inference}
\label{sec:parallel}
Baseline PixelCNN method can enjoy parallel inference for multiple images supported by graphic process unit (GPU), as other deep learning algorithms. 
In the proposed Skim-PixelCNN, the parallel inference is little tricky because the skimming decision for the pixel should be different among images.
Therefore, to utilize the parallel calculation, we uniformly use a confidence map which is a maximum of the confidence map for every images in the batch. 
Clearly, this is the upper bound of the skimming and does not harm the generation performance. 
However, PixelCNN sometimes inevitably samples unsuccessful images and in this case, the Skim-PixelCNN cannot sufficiently skim the region.
To avoid the situation, we set the final confidence value of the pixel as an upper few percentile of the all the confidence value of the pixel for every batch.
Figure shows the example of the images. From the results, we confirmed that this parallelization does not harm the generation quality of the proposed method.
Table \ref{table:parallel_inference} shows inference time (except anchors) speedup and skimming ratio for varying $\eps$ and percentiles.

\begin{table}[t]
\centering
\caption{Inference time speedup (IT), inference time except anchors speedup (IT \textbackslash{}A), skimming ratio (SR) for varying $\eps$ and percentile, batch size = 100, we report average of experiments.}
\label{table:parallel_inference}

\vspace{2mm}

\begin{tabular}{ll}
\toprule
%                             &  PixelCNN++ \cite{salimans2017pixelcnn++} \\
                              &  PixelCNN++                               \\
\midrule
Inference Time                &  27785.1 sec (7 hour 41 min)              \\
Inference Time except anchors &  26048.5 sec (7 hour 14 min)              \\
\bottomrule

\vspace{1mm}

\end{tabular}

\begin{tabular}{l|lll|lll|lll}
\toprule
           & \multicolumn{3}{c|}{$\eps = 0.9$}        & \multicolumn{3}{c|}{$\eps = 0.8$}        & \multicolumn{3}{c}{$\eps = 0.7$}  \\
\midrule
Percentile & IT    & IT \textbackslash{}A & SR    & IT    & IT \textbackslash{}A & SR    & IT    & IT \textbackslash{}A & SR  \\
\midrule
1.0 (max)  & 1.4x  & 1.4x  & 30.8  & 1.3x  & 1.3x  & 23.6  & 1.2x  & 1.2x  & 15.5 \\
0.9        & 3.5x  & 4.2x  & 77.9  & 3.0x  & 3.5x  & 72.8  & 2.4x  & 2.6x  & 63.6 \\
0.8        & 5.8x  & 8.6x  & 89.9  & 4.3x  & 5.6x  & 83.7  & 3.2x  & 3.8x  & 74.9 \\
0.7        & 7.1x  & 12.0x & 93.3  & 5.9x  & 8.7x  & 90.1  & 4.4x  & 5.7x  & 83.9 \\
0.6        & 8.0x  & 15.0x & 94.9  & 6.5x  & 10.4x & 92.0  & 5.4x  & 7.7x  & 88.7 \\
0.5 (median) & 8.9x  & 18.7x & 96.2  & 7.2x  & 12.4x & 93.5  & 6.4x  & 10.0x & 91.6 \\
0.4        & 9.2x  & 20.2x & 96.6  & 7.9x  & 14.8x & 94.8  & 6.9x  & 11.4x & 92.8 \\
0.3        & 10.0x & 25.2x & 97.6  & 8.8x  & 18.2x & 96.1  & 7.5x  & 13.4x & 94.1 \\
0.2        & 10.9x & 32.2x & 98.5  & 9.3x  & 20.7x & 96.7  & 8.2x  & 15.9x & 95.3 \\
0.1        & 11.9x & 43.7x & 99.3  & 10.8x & 30.9x & 98.3  & 9.7x  & 23.0x & 97.2 \\
0.0 (min)  & 12.9x & 63.0x & 100.0 & 12.9x & 62.4x & 100.0 & 12.6x & 56.7x & 99.8 \\
\bottomrule
\end{tabular}

\vspace{2mm}

\begin{tabular}{l|lll|lll|lll}
\toprule
           & \multicolumn{3}{c|}{$\eps = 0.6$}        & \multicolumn{3}{c|}{$\eps = 0.5$}        & \multicolumn{3}{c}{$\eps = 0.4$}  \\
\midrule
Percentile & IT    & IT \textbackslash{}A & SR    & IT    & IT \textbackslash{}A & SR    & IT    & IT \textbackslash{}A & SR  \\
\midrule
1.0 (max)    & 1.0x  & 1.0x  & 3.2  & 1.0x & 1.0x  & 4.1  & 1.0x & 1.0x & 1.3  \\
0.9          & 2.2x  & 2.3x  & 58.8 & 1.8x & 1.9x  & 48.3 & 1.5x & 1.5x & 36.1 \\
0.8          & 2.7x  & 3.1x  & 69.0 & 2.2x & 2.4x  & 60.8 & 1.7x & 1.8x & 45.1 \\
0.7          & 3.3x  & 3.9x  & 75.9 & 2.6x & 2.9x  & 67.0 & 2.2x & 2.4x & 59.1 \\
0.6          & 4.1x  & 5.2x  & 82.3 & 3.1x & 3.6x  & 73.7 & 2.4x & 2.7x & 64.7 \\
0.5 (median) & 4.9x  & 6.7x  & 86.6 & 3.7x & 4.5x  & 79.4 & 2.8x & 3.1x & 69.8 \\
0.4          & 5.8x  & 8.6x  & 89.9 & 4.5x & 5.8x  & 84.3 & 3.3x & 3.9x & 75.7 \\
0.3          & 6.6x  & 10.6x & 92.2 & 5.2x & 7.3x  & 87.9 & 3.9x & 4.8x & 80.8 \\
0.2          & 7.5x  & 13.3x & 94.1 & 6.3x & 9.8x  & 91.4 & 4.6x & 6.1x & 85.2 \\
0.1          & 8.7x  & 18.0x & 96.0 & 7.4x & 13.1x & 93.9 & 6.1x & 9.3x & 90.8 \\
0.0 (min)    & 12.3x & 49.5x & 99.6 & 11.1 & 34.3  & 98.7 & 10.1 & 25.4 & 97.6 \\
\bottomrule
\end{tabular}
\end{table}

\subsection{Faster generation}
To show that our module can be easily combined on top of the other pixelCNN variants, we incorporated our skimming method to the fast version of the PixelCNN++ algorithm~\citep{ramachandran2017fast}. Fast PixelCNN++ is the state-of-the-art (SOTA) among the PixelCNN variants that caches the previously gathered information to enhance the generation speed. Table~\ref{table:speedup_performance2} shows the generation time using the incorporated model (\emph{skim}+Fast PixelCNN++). 
%Due to the lack of time to fully investigate all datasets with the new implementation, we conducted the experiment on CIFAR-10, which is the most widely used dataset in PixelCNN works and is more diverse than the CelebA dataset. 
It is noteworthy that we could further push the limit beyond the speed of the baseline algorithm by incorporating the proposed skimming module. From the results, we showed the fastest generation performance of the kind. Generated CIFAR-10 samples by (\emph{skim}+Fast PixelCNN++) are in Appendix~\ref{app:add}.
From the images, we confirmed that the proposed method could generated image with skimming, despite that CIFAR-10 is more difficult to learn where to skim compared to CelebA because of its diverse objects and patterns. 

\begin{table}[t]
\tabcolsep=0.15cm
\centering
    \caption{The generation time per image and the skimming ratio over $\epsilon$ using Fast-PixelCNN++~\citep{ramachandran2017fast}. CelebA is tested with the image size of 32$\times$32 to compare CIFAR-10. The generation time of Fast-PixelCNN++ (1.0x) is \textbf{23.8} sec. 
    %\yj{change celeb 32$\times$32 with celeb 64$\times$64. - wed}
    }
\label{table:speedup_performance2}
\vspace{-2mm}
\begin{tabular}{l|llllll|llllll}
\toprule
Dataset &\multicolumn{6}{c|}{CIFAR-10 $32\times32$} & \multicolumn{6}{c}{CelebA $32\times32$} \\
\midrule
\toprule
$\epsilon$               & 0.0 & 0.2  & 0.4  & 0.6  & 0.8  & 1.0  & 0.0 & 0.2  & 0.4  & 0.6  & 0.8   & 1.0   \\
\midrule
\sd{SU}                   & 1.0x & 1.2x & 1.4x & 1.6x & 2.1x & 4.9x & 1.0x &1.5x & 2.9x & 4.2x & 4.6x  & 4.9x \\
\sd{SU} \textbackslash{}A & 1.0x & 1.2x & 1.5x & 1.7x & 2.4x & 11.1x & 1.0x &1.6x & 3.2x & 4.3x & 6.8x & 11.1x \\
SR (\%)              & 0.00 & 24.9 & 36.5 & 43.7 & 57.0 & 87.5 & 0.00 & 41.0 & 64.8 & 77.8 & 83.2 & 87.5 \\
\bottomrule
\end{tabular}
\end{table}

\subsection{More Selected Results}
In addition to the results presented in the paper, we shows supplement generation examples in below figures.
Figure~\ref{fig:more_selected_0} and \ref{fig:more_selected_1} shows the additional facial image generation  results by Skim-PixelCNN among $\eps \in [1.0, 0.0]$. In Figure~\ref{fig:imagenet_1} and \ref{fig:imagenet_2}, additional ImageNet generation examples are presented with larger image size. 
Also, we shows the generation results with parallel inference in Figure~\ref{fig:parallel_result}, which follows the method described in Section~\ref{sec:parallel}. 
%Figure \ref{fig:more_selected_0} and \ref{fig:more_selected_1} show selected generated images 

\begin{figure}[t!]
\begin{center}
   \includegraphics[width=0.99\linewidth]{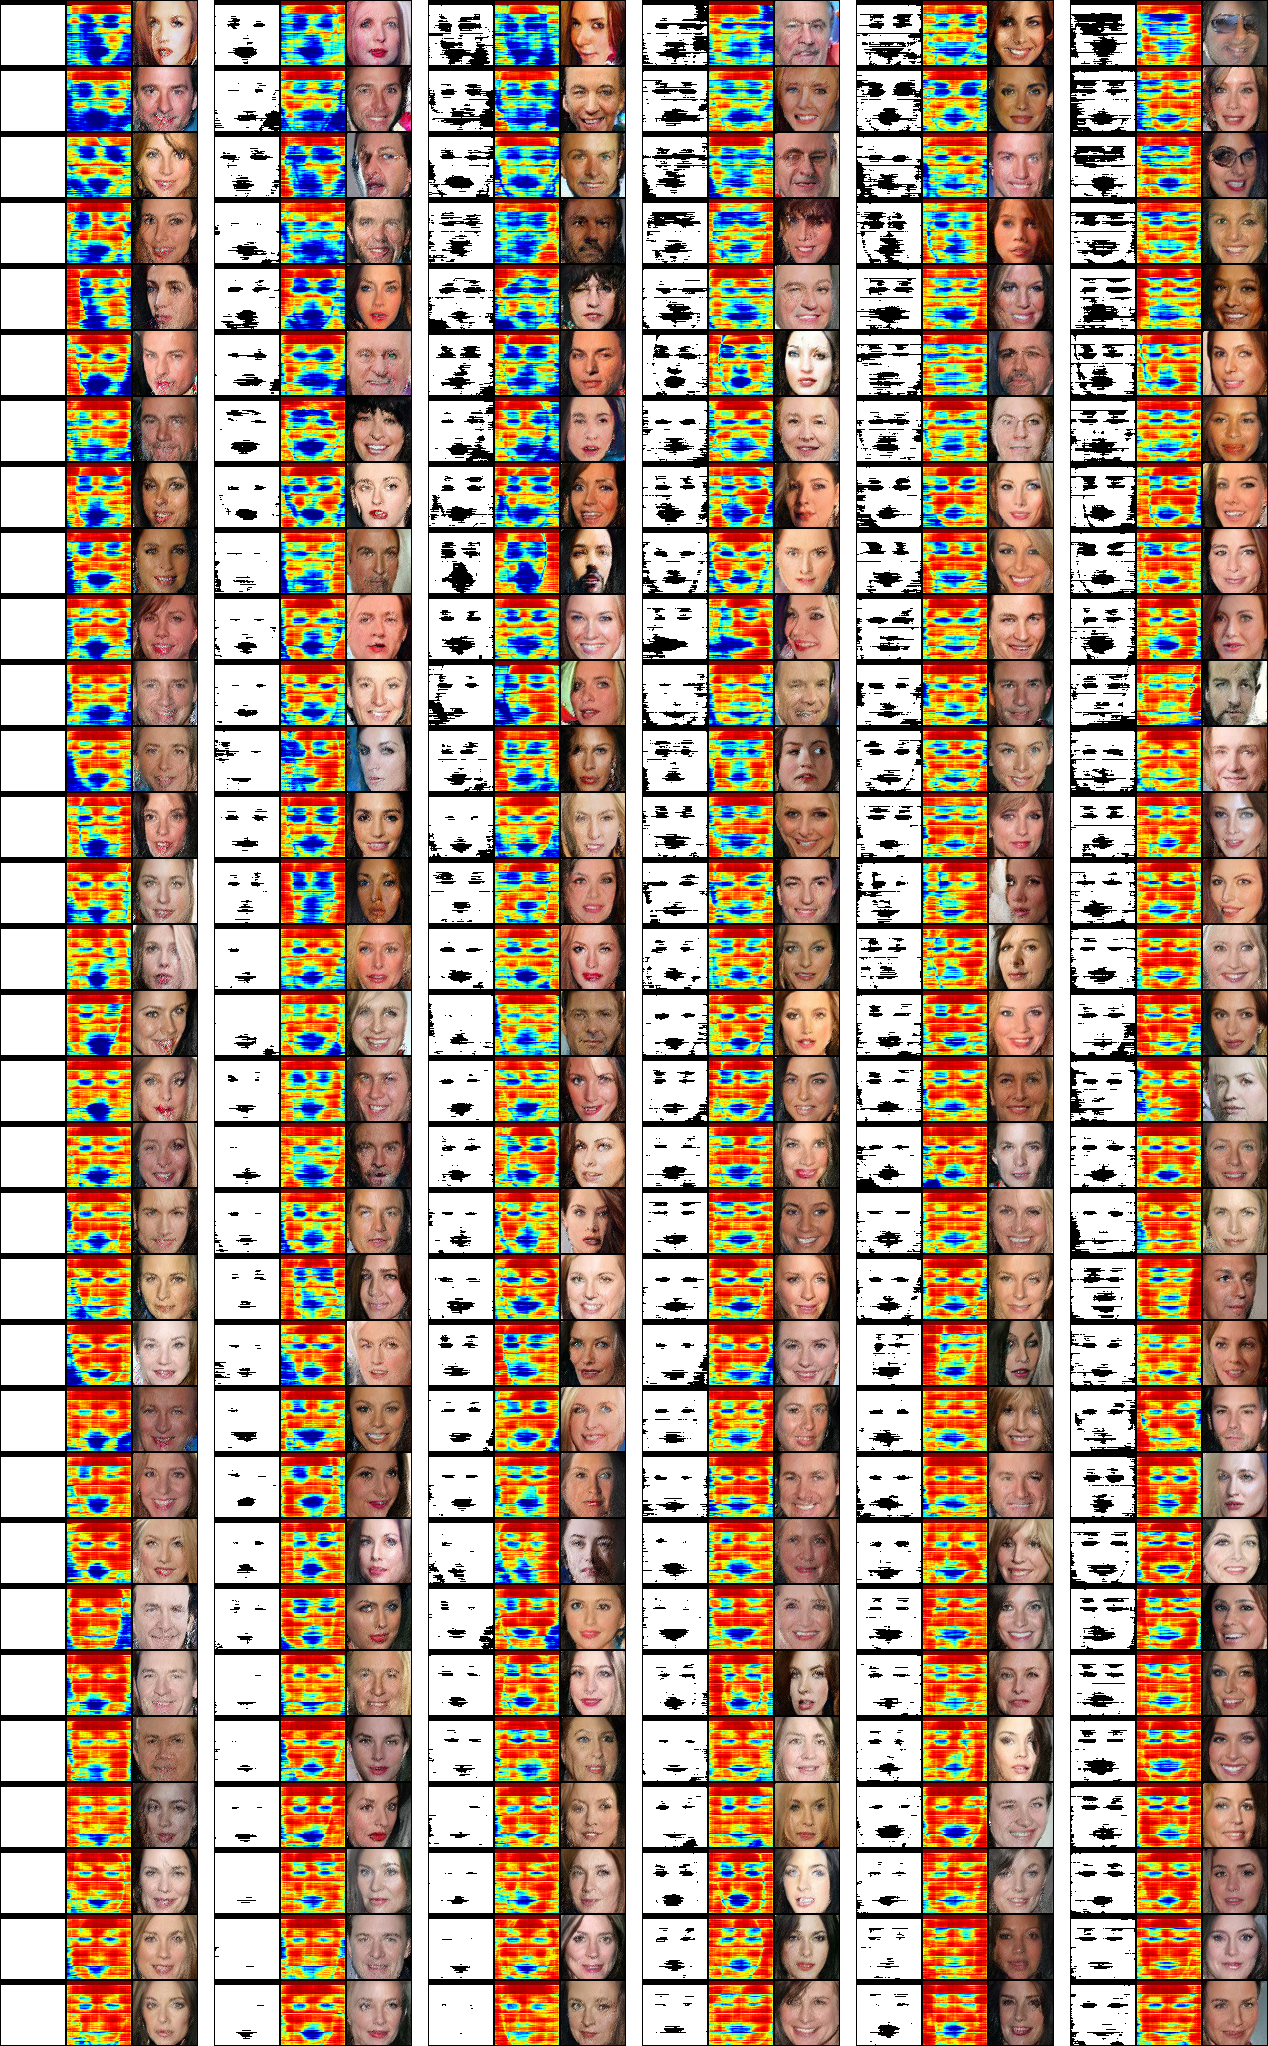}
\end{center}
   \caption{More selected CelebA generation result in $64\times64$. according to $\eps \in \{1.0, 0.9, 0.8, 0.7, 0.6, 0.5 \}$.}
\label{fig:more_selected_0}
\end{figure}

\begin{figure}[t!]
\begin{center}
   \includegraphics[width=0.84\linewidth]{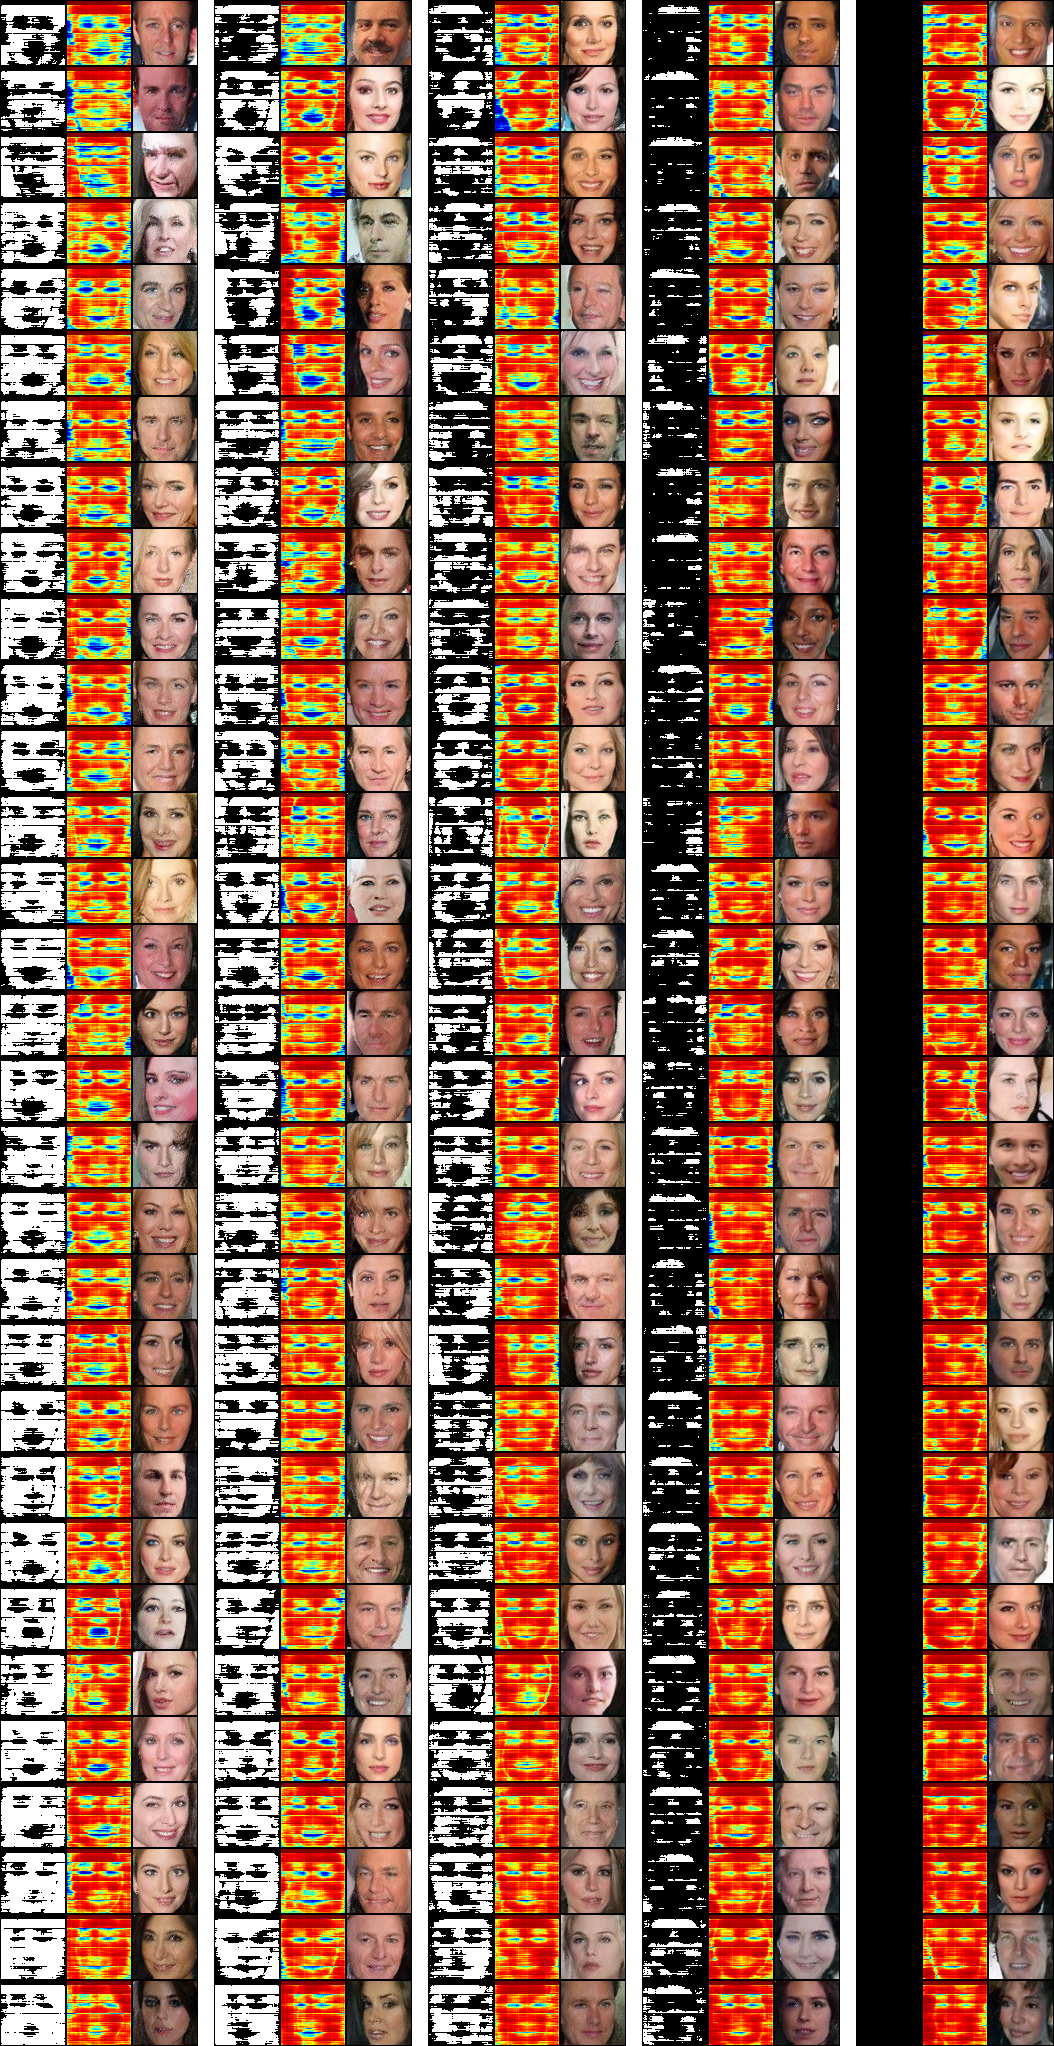}
\end{center}
   \caption{More selected CelebA generation result in $64\times64$. according to $\eps \in \{0.4, 0.3, 0.2, 0.1, 0.0\} $.}
\label{fig:more_selected_1}
\end{figure}

\iffalse
\begin{figure}[t!]
\begin{center}
   \includegraphics[width=0.99\linewidth]{Images/sup_failed.pdf}
\end{center}
   \caption{Selected failed generation cases using CelebA $64\times64$ model according to $\eps \in \{1.0, 0.9, 0.8, 0.7, 0.6, 0.5\}$.}
\end{figure}
\fi

\begin{figure}[t]
\centering
%\begin{subfigure}[t]{0.24\textwidth}
\begin{subfigure}[t]{0.99\textwidth}
\includegraphics[width=\linewidth]{Images/balloonflower.png}
\caption{Balloon Flower} \label{fig:imagenet1}
\end{subfigure}\hfill
\begin{subfigure}[t]{0.99\textwidth}
\includegraphics[width=\linewidth]{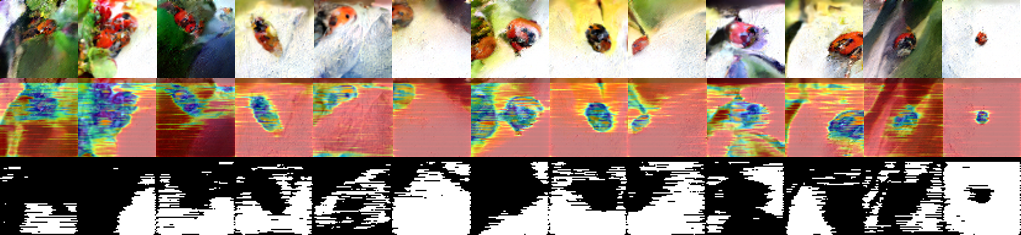}
\caption{Ladybug} \label{fig:imagenet2}
\end{subfigure}\hfill
\begin{subfigure}[t]{0.99\textwidth}
\includegraphics[width=\linewidth]{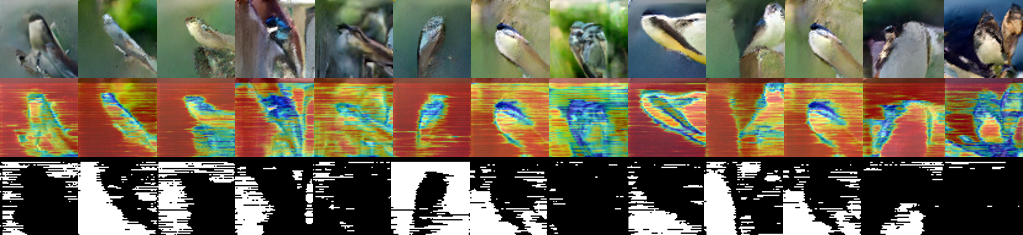}
\caption{Tree-martin} \label{fig:imagenet3}
\end{subfigure}\hfill
\begin{subfigure}[t]{0.99\textwidth}
\includegraphics[width=\linewidth]{Images/pizza.png}
\caption{Pizza} \label{fig:imagenet4}
\end{subfigure}\hfill
%\begin{center}
%   \includegraphics[width=0.55\linewidth]{Images/attention_vs_time.pdf}
%\end{center}
   \caption{ImageNet generation examples (1).}
   \label{fig:imagenet_1}
   %\vspace{-2mm}
\end{figure}

\begin{figure}[t]
\centering
%\begin{subfigure}[t]{0.24\textwidth}
\begin{subfigure}[t]{0.99\textwidth}
\includegraphics[width=\linewidth]{Images/sorrel.png}
\caption{Sorrel} \label{fig:imagenet1}
\end{subfigure}\hfill
\begin{subfigure}[t]{0.99\textwidth}
\includegraphics[width=\linewidth]{Images/bear.png}
\caption{Brown bear} \label{fig:imagenet2}
\end{subfigure}\hfill
\begin{subfigure}[t]{0.99\textwidth}
\includegraphics[width=\linewidth]{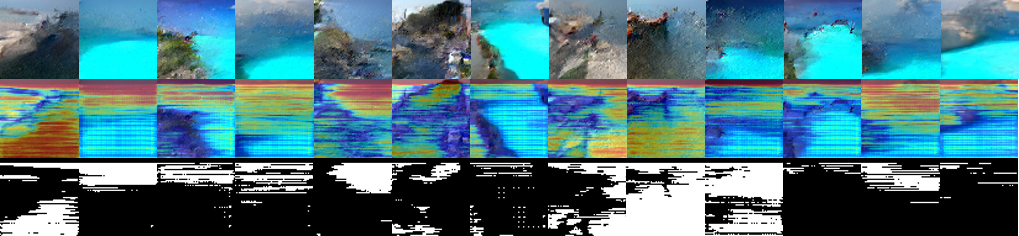}
\caption{Sandbar} \label{fig:imagenet3}
\end{subfigure}\hfill
\begin{subfigure}[t]{0.99\textwidth}
\includegraphics[width=\linewidth]{Images/coral.png}
\caption{Coral} \label{fig:imagenet4}
\end{subfigure}\hfill
%\begin{center}
%   \includegraphics[width=0.55\linewidth]{Images/attention_vs_time.pdf}
%\end{center}
   \caption{ImageNet generation examples (2).}
   \label{fig:imagenet_2}
   %\vspace{-2mm}
\end{figure}

\begin{figure}[t]
\centering
%\begin{subfigure}[t]{0.24\textwidth}
\begin{subfigure}[t]{0.24\textwidth}
\includegraphics[width=\linewidth]{Images/exp_balloon.png}
\caption{Balloon Flower} \label{fig:imagenet1}
\end{subfigure}\hfill
\begin{subfigure}[t]{0.24\textwidth}
\includegraphics[width=\linewidth]{Images/exp_ladybug.png}
\caption{Ladybug} \label{fig:imagenet2}
\end{subfigure}\hfill
\begin{subfigure}[t]{0.24\textwidth}
\includegraphics[width=\linewidth]{Images/exp_treemartin.png}
\caption{Tree-martin} \label{fig:imagenet3}
\end{subfigure}\hfill
\begin{subfigure}[t]{0.24\textwidth}
\includegraphics[width=\linewidth]{Images/exp_pizza.png}
\caption{Pizza} \label{fig:imagenet4}
\end{subfigure}\hfill
\begin{subfigure}[t]{0.24\textwidth}
\includegraphics[width=\linewidth]{Images/exp_sorrel.png}
\caption{Sorrel} \label{fig:imagenet5}
\end{subfigure}\hfill
\begin{subfigure}[t]{0.24\textwidth}
\includegraphics[width=\linewidth]{Images/exp_bear.png}
\caption{Brown bear} \label{fig:imagenet6}
\end{subfigure}\hfill
\begin{subfigure}[t]{0.24\textwidth}
\includegraphics[width=\linewidth]{Images/exp_sandbar.png}
\caption{Sandbar} \label{fig:imagenet7}
\end{subfigure}\hfill
\begin{subfigure}[t]{0.24\textwidth}
\includegraphics[width=\linewidth]{Images/exp_coral.png}
\caption{Coral reef} \label{fig:imagenet8}
\end{subfigure}\hfill
%\begin{center}
%   \includegraphics[width=0.55\linewidth]{Images/attention_vs_time.pdf}
%\end{center}
   \caption{ImageNet generation examples (3).}
   \label{fig:exp_imagenet}
   %\vspace{-2mm}
\end{figure}

\begin{figure}[t!]
\begin{center}
   \includegraphics[width=0.99\linewidth]{Images/sup_parallel_pixelcnn.png}
\end{center}
   \caption{Generated images by PixelCNN++ with batch size 100}
\end{figure}

\begin{figure}[t!]
\centering
\begin{subfigure}[t]{0.45\textwidth}
\includegraphics[width=\linewidth]{Images/sup_t4p9h.png}
\caption{Attention heatmap for $\eps = 0.4$ and $p = 90$.}
\end{subfigure}
\begin{subfigure}[t]{0.45\textwidth}
\includegraphics[width=\linewidth]{Images/sup_t4p9s.png}
\caption{Generated images for $\eps = 0.4$ and $p = 90$.} \label{fig:sup_parallel_1}
\end{subfigure}

\begin{subfigure}[t]{0.45\textwidth}
\includegraphics[width=\linewidth]{Images/sup_t8p9h.png}
\caption{Attention heatmap for $\eps = 0.8$ and $p = 90$.}
\end{subfigure}
\begin{subfigure}[t]{0.45\textwidth}
\includegraphics[width=\linewidth]{Images/sup_t8p9s.png}
\caption{Generated images for $\eps = 0.8$ and $p = 90$.} \label{fig:sup_parallel_3}
\end{subfigure}

\begin{subfigure}[t]{0.45\textwidth}
\includegraphics[width=\linewidth]{Images/sup_t4p3h.png}
\caption{Attention heatmap for $\eps = 0.4$ and $p = 30$.}
\end{subfigure}
\begin{subfigure}[t]{0.45\textwidth}
\includegraphics[width=\linewidth]{Images/sup_t4p3s.png}
\caption{Generated images for $\eps = 0.4$ and $p = 30$.} \label{fig:sup_parallel_2}
\end{subfigure}

\begin{subfigure}[t]{0.3\textwidth}
\centering
\includegraphics[width=0.33\linewidth]{Images/sup_t4p9m.png}
\caption{Skimmed region of \ref{fig:sup_parallel_1}.}
\end{subfigure}
\begin{subfigure}[t]{0.3\textwidth}
\centering
\includegraphics[width=0.33\linewidth]{Images/sup_t8p9m.png}
\caption{Skimmed region of \ref{fig:sup_parallel_3}.}
\end{subfigure}
\begin{subfigure}[t]{0.3\textwidth}
\centering
\includegraphics[width=0.33\linewidth]{Images/sup_t4p3m.png}
\caption{Skimmed region of \ref{fig:sup_parallel_2}.}
\end{subfigure}
\caption{Confidence map, generated images and skimmed region for varying parameters with batch size = 100.}
\label{fig:parallel_result}
\end{figure}
